# Supplementary material for: CLOSER: Towards Better Representation Learning for Few-Shot Class-Incremental Learning
Source: arXiv:2410.05627 source file (2024-10-08)
Supplement: Supplementary file 1 [file intra_inter.tex]

\section{Comparison between Reducing Intra-Class and Inter-Class Distance}\label{supp:sec:intra_inter}
As discussed in Section~\textcolor{red}{3.4}, the dispersion of the representations leads to the performance decline in the classifier replacement (CR) process, since it becomes challenging for the class prototype to adequately represent the scattered features via averaging.
One na\"ive solution is to directly suppress the intra-class distribution, which can be implemented by minimizing the intra-class distance:
\begin{equation}
    \mathcal{L}_{\text{intra}} = - \frac{1}{\sum\limits_{i=1}^B \sum\limits_{j>i}^B \mathbbm{1}_{[y_i = y_j]}} \sum\limits_{i=1}^B \sum\limits_{j>i}^B \mathbbm{1}_{[y_i = y_j]} \texttt{sim}(\vz_i,\vz_j).
\end{equation}
However, we find that directly reducing intra-class distance has negative influences on the performance on both base and new classes, as demonstrated in Fig.~\ref{fig:supp:intra_inter} and Table~\ref{tab:supp:intra_inter}.
One possible explanation is that reducing intra-class distribution may adversely affect the representation generalization ability by impeding its capacity to capture fine-grained details among different instances.
This is supported by the largely degraded performance
results presented in both Fig.~\ref{fig:supp:intra_inter} and the results on CUB200 in Table~\ref{tab:supp:intra_inter}, particularly considering the limited number of training examples in CUB200 and its fine-grained-class property.
On the contrary, reducing inter-class distance is observed to achieve outstanding performance both on base and new classes, which validates our assertion on reducing inter-class distance.
%when the distance between classes diminishes, it enables the acquisition of shared information between classes, as a similar concept is discussed in~\cite{zou2022margin} regarding the negative margin in the softmax function.

\begin{figure}
    \centering
    \includegraphics[width=0.45\textwidth]{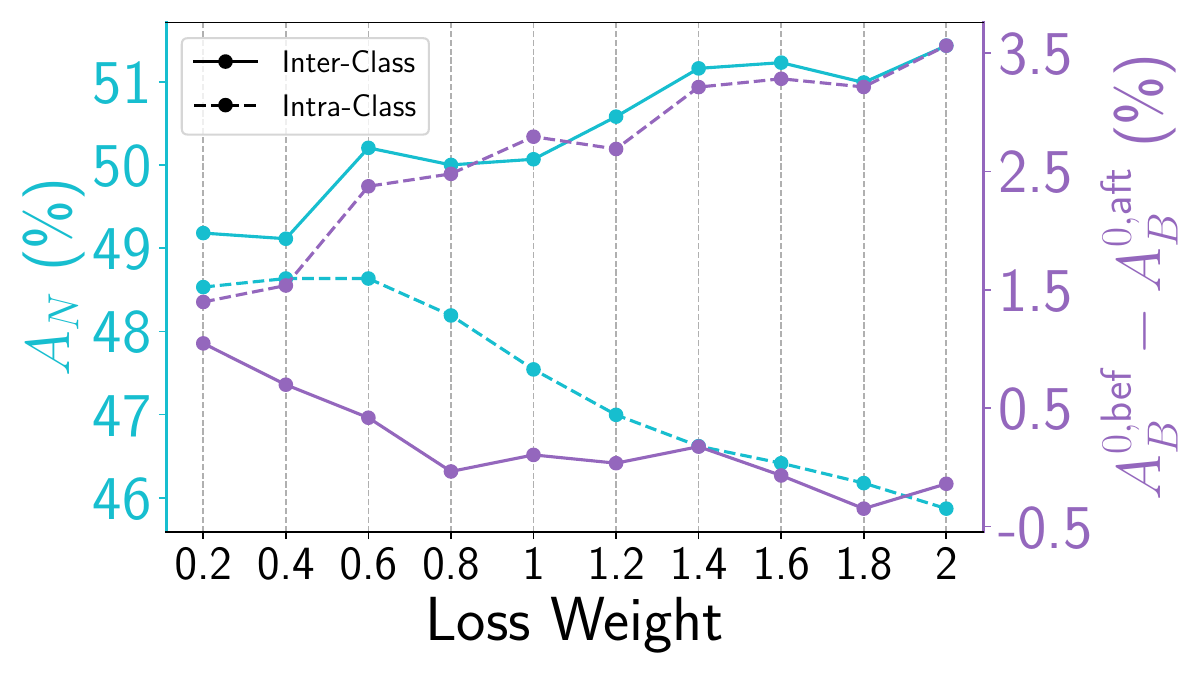}
    \caption{\textbf{Comparison between the impact of reducing intra-class and inter-class distance.}
    Reducing intra-class distance harms the performance on new classes (\textcolor{SkyBlue}{dotted sky blue line}) and exacerbates the performance drop from classifier replacement (CR) (\textcolor{violet}{dotted purple line}).
    Conversely, reducing inter-class distance benefits new-class accuracy (\textcolor{SkyBlue}{solid sky blue line}) and alleviates the performance degradation from CR (\textcolor{violet}{solid purple line}).
    The experiments are conducted on CUB200 dataset.
    }
    \label{fig:supp:intra_inter}
\end{figure}
