# Supplementary material for: CLOSER: Towards Better Representation Learning for Few-Shot Class-Incremental Learning
Source: arXiv:2410.05627 source file (2024-10-08)
Supplement: Supplementary file 2 [file intra_inter.tex]

\begin{figure}
    \centering
    \includegraphics[width=0.45\textwidth]{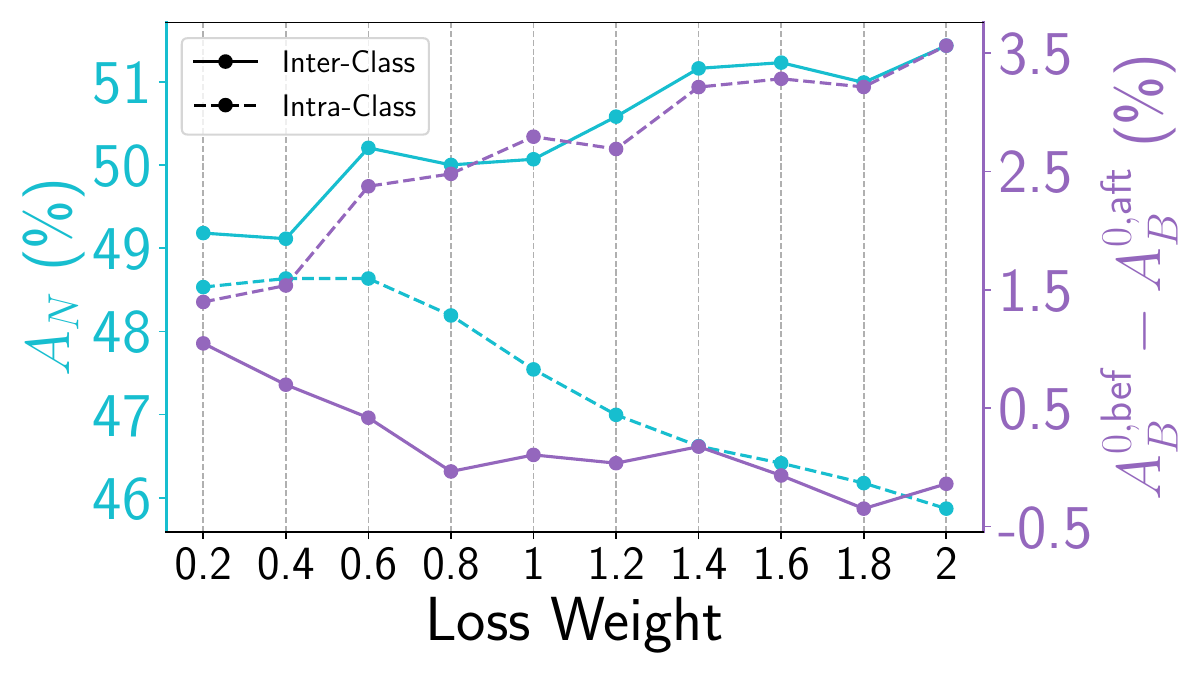}
    \caption{\textbf{Comparison between the impact of reducing intra-class and inter-class distance.}
    Reducing intra-class distance harms the performance on new classes (\textcolor{SkyBlue}{dotted sky blue line}) and exacerbates the performance drop from classifier replacement (CR) (\textcolor{violet}{dotted purple line}).
    Conversely, reducing inter-class distance benefits new-class accuracy (\textcolor{SkyBlue}{solid sky blue line}) and alleviates the performance degradation from CR (\textcolor{violet}{solid purple line}).
    The experiments are conducted on CUB200 dataset.
    }
    \label{fig:supp:intra_inter}
\end{figure}
