# Supplementary material for: CLOSER: Towards Better Representation Learning for Few-Shot Class-Incremental Learning
Source: arXiv:2410.05627 source file (2024-10-08)
Supplement: Supplementary file 3 [file intra_inter.tex]

\begin{table}[t!]
\centering
\small
\caption{\textbf{Comparison between the impact of reducing intra-class and inter-class distance.}
    `Inter-class*' means that the minimization is carried out on a subset of inter-class pairs, which is chosen to have an equal number as the intra-class pairs, ensuring a fair comparison.
    }
\resizebox{0.6\linewidth}{!}{
    \begin{tabular}{lccccc}
      \toprule
      %\multirow{2}{*}{DA.} & \multirow{2}{*}{\textit{low} $\tau$}& \multirow{2}{*}{$\mathcal{L}_{\text{infoNCE}}$} & \multirow{2}{*}{$\mathcal{L}_{cos}$} & \multicolumn{3}{c}{Acc. (\%)} & \multirow{2}{*}{PD. $\downarrow$}\\
      Dataset & Minimization & $A_B$ & $A_N$ & $A_W$ & $A_B^{0,\text{bef}}$-$A_B^{0,\text{aft}}$\\
      \toprule
      \multirow{3}{*}{\small CIFAR100} & Intra-class&68.78&24.30&50.99&2.71\\
      &Inter-class*&70.32&\textbf{27.28}&53.10&\textbf{1.31}\\
      &Inter-class&\textbf{70.72}&27.23&\textbf{53.32}&1.58\\
      \midrule
      \multirow{3}{*}{\small \textit{mini}ImageNet} & Intra-class&71.17&24.10&52.34&0.43\\
      &Inter-class*&71.85&24.48&52.90&0.34\\
      &Inter-class&\textbf{72.03}&\textbf{25.28}&\textbf{53.33}&\textbf{0.21}\\
      \midrule
      \multirow{3}{*}{\small CUB200} & Intra-class&73.12&46.45&59.63&2.58\\
      &Inter-class*&\textbf{76.47}&\textbf{51.47}&\textbf{63.83}&\textbf{0.58}\\
      &Inter-class&76.40&51.06&63.58&0.62\\
      \bottomrule
    \end{tabular}}
    \label{tab:supp:intra_inter}
\end{table}
